# Supplementary material for: Analytic gradients for equation-of-motion coupled cluster with single, double, and perturbative triple excitations
Source: arXiv:2406.05595 ancillary file (2024-06-08)
Supplement: Supplementary file 1 [file SI.pdf]

# Supporting Information: Analytic gradients for equation-of-motion coupled cluster with single, double, and perturbative triple excitations

Tingting Zhao and Devin. A. Matthews*

*Department of Chemistry, Southern Methodist University, Dallas, TX 75275, United States*

E-mail: dmatthews@smu.edu

## Geometries

The optimized ground states and excited states geometries for all three systems are presented in geometries.xlsx.

## Validation

TABLE 1. Gradients in Hartree/bohr and Hartree/radian along internal coordinates calculated by analytic derivative (AD) and finite differences (FD) with the aug-cc-pVDZ basis set for $1^1A_2(n \to \pi^*)$ valence excited state of formaldehyde at ground state geometry obtained from the QUEST2 dataset.[1]

| Parameter | $r_{C-O}$ | $r_{C-H}$ | $\angle_{C-O-H}$ | $\phi$ |
|---|---|---|---|---|
| AD | -0.1566619756 | -0.0069335888 | 0.0057434601 | 0.0009551133 |
| FD | -0.1566622971 | -0.0069338812 | 0.0057437959 | 0.0009550812 |

# Supplement data for cytosine system

TABLE 2. Gradients and parameter values at the last geometry optimization step with RMS force of 0.000004045 for cytosine with EOM-CCSD/cc-pVDZ. Gradients are reported in Hartree/bohr and Hartree/radian, and parameter values are reported in angstroms and degrees.

| Parameter | dV/dR | Step | Rold | Rnew |
|---|---|---|---|---|
| $r_{C_2-N_1}$ | 0.0000036126 | -0.0000008004 | 1.4168672753 | 1.4168664750 |
| $r_{N_3-C_2}$ | 0.0000034926 | -0.0000020169 | 1.3762915433 | 1.3762895264 |
| $r_{H_4-N_3}$ | 0.0000021680 | -0.0000015797 | 1.0079395385 | 1.0079379589 |
| $r_{H_5-N_3}$ | 0.0000018888 | -0.0000012514 | 1.0090011500 | 1.0089998986 |
| $r_{C_6-N_1}$ | -0.0000037096 | -0.0000027388 | 1.3233461840 | 1.3233434452 |
| $r_{O_7-C_6}$ | -0.0000021864 | 0.0000061874 | 1.2693136827 | 1.2693198700 |
| $r_{N_8-C_6}$ | 0.0000003512 | -0.0000049042 | 1.4097212968 | 1.4097163926 |
| $r_{H_9-N_8}$ | 0.0000031539 | -0.0000022667 | 1.0146954721 | 1.0146932054 |
| $r_{C_{10}-N_8}$ | 0.0000016023 | 0.0000006093 | 1.3835214366 | 1.3835220459 |
| $r_{H_{11}-C_{10}}$ | 0.0000006310 | 0.0000000170 | 1.0893217107 | 1.0893217277 |
| $r_{C_{12}-C_{10}}$ | -0.0000027502 | 0.0000041368 | 1.4358168294 | 1.4358209662 |
| $r_{H_{13}-C_{12}}$ | -0.0000009047 | 0.0000016361 | 1.0940623563 | 1.0940639924 |
| $\angle_{N_1-C_2-N_3}$ | -0.0000002253 | -0.0001201251 | 112.2030602057 | 112.2029400806 |
| $\angle_{C_2-N_3-H_4}$ | 0.0000001601 | -0.0001194636 | 121.9910126603 | 121.9908931967 |
| $\angle_{C_2-N_3-H_5}$ | -0.0000011201 | 0.0003137785 | 117.8227782260 | 117.8230920045 |
| $\angle_{C_2-N_1-C_6}$ | -0.0000080923 | -0.0000260229 | 116.0784443779 | 116.0784183550 |
| $\angle_{N_1-C_6-O_7}$ | 0.0000006523 | -0.0003342175 | 123.5284401924 | 123.5281059748 |
| $\angle_{N_1-C_6-N_8}$ | -0.0000136198 | 0.0004999776 | 123.6348613900 | 123.6353613676 |
| $\angle_{C_6-N_8-H_9}$ | 0.0000003543 | -0.0000122045 | 115.4752989824 | 115.4752867779 |
| $\angle_{C_6-N_8-C_{10}}$ | -0.0000119719 | -0.0002573662 | 121.7767987646 | 121.7765413984 |
| $\angle_{N_8-C_{10}-H_{11}}$ | -0.0000007598 | 0.0002652432 | 118.7078025695 | 118.7080678127 |
| $\angle_{N_8-C_{10}-C_{12}}$ | -0.0000056794 | 0.0001598417 | 115.9150903775 | 115.9152502192 |
| $\angle_{C_{10}-C_{12}-H_{13}}$ | 0.0000000668 | -0.0000397441 | 119.1160627321 | 119.1160229879 |
| $\phi_{N_1-C_2-N_3-H_4}$ | 0.0000034085 | -0.0026239386 | 179.9938781370 | 179.9912541984 |
| $\phi_{N_1-C_2-N_3-H_5}$ | -0.0000031027 | 0.0025410490 | 0.0080335248 | 0.0105745738 |
| $\phi_{C_6-N_1-C_2-N_3}$ | 0.0000020463 | -0.0007763326 | 179.9987065186 | 179.9979301860 |
| $\phi_{C_2-N_1-C_6-O_7}$ | -0.0000013737 | 0.0005502535 | -180.0000000000 | 179.9994497465 |
| $\phi_{C_2-N_1-C_6-N_7}$ | 0.0000028789 | -0.0009734844 | 0.0014115109 | 0.0004380266 |
| $\phi_{N_1-C_6-N_8-H_9}$ | 0.0000002562 | -0.0001873247 | -179.9981668754 | 179.9983542001 |
| $\phi_{N_1-C_6-N_8-C_{10}}$ | -0.0000000587 | 0.0004482050 | 0.0000000000 | 0.0004482050 |
| $\phi_{C_6-N_8-C_{10}-H_{11}}$ | 0.0000000239 | -0.0000682270 | 180.0000000000 | 179.9999317730 |
| $\phi_{C_6-N_8-C_{10}-C_{12}}$ | -0.0000009994 | 0.0008141789 | 0.0000000000 | 0.0008141789 |
| $\phi_{N_8-C_{10}-C_{12}-H_{13}}$ | -0.0000008145 | 0.0006641527 | 180.0000000000 | 180.0006641527 |

TABLE 3. Harmonic vibrational frequencies ($\omega$), infrared intensities ($I$) for the $1^1A'$ state of cytosine calculated with EOM-CCSD/cc-pVDZ. The converged EOM-CCSD* geometry was used.

| $\omega$ ($cm^{-1}$) | $I$ (km/mol) | $\omega$ ($cm^{-1}$) | $I$ (km/mol) |
|---|---|---|---|
| 3675.4645 | 98.3786 | 930.6409 | 26.3611 |
| 3648.2126 | 8.5948 | 807.0303 | 189.15 |
| 3535.3495 | 7.9567 | 781.8734 | 24.8847 |
| 3272.4947 | 0.6273 | 747.7156 | 195.198 |
| 3211.9746 | 11.2503 | 719.4268 | 6.0284 |
| 1666.8478 | 152.5941 | 570.5505 | 8.4879 |
| 1651.9080 | 155.7694 | 543.5701 | 43.8674 |
| 1605.5302 | 18.7358 | 511.6984 | 24.2124 |
| 1500.8382 | 9.7078 | 507.5224 | 19.9646 |
| 1424.0685 | 11.2547 | 476.9967 | 28.2281 |
| 1360.6998 | 43.3123 | 427.3808 | 42.0967 |
| 1304.6058 | 43.7476 | 354.6183 | 2.7867 |
| 1208.2259 | 5.3603 | 342.3579 | 6.3265 |
| 1140.2795 | 0.0838 | 297.9162 | 25.1929 |
| 1052.7688 | 48.2249 | 197.0304 | 12.7345 |
| 1024.1761 | 11.5626 | 128.0550 | 8.8205 |
| 1007.0577 | 13.6039 | | |

# References

(1) Loos, P.-F.; Boggio-Pasqua, M.; Scemama, A.; Caffarel, M.; Jacquemin, D. Reference Energies for Double Excitations. *Journal of Chemical Theory and Computation* **2019**, *15*, 1939–1956.
